# Supplementary material for: Almost AI, Almost Human: The Challenge of Detecting AI-Polished Writing
Source: arXiv:2502.15666 source file (2025-05-05)
Supplement: Supplementary file 1 [file appendix.tex]

\subsection{Dataset}
\input{latex/app/dataset}

\newpage
\subsection{Detectors}
\input{latex/app/detector}

\newpage
\subsection{Results}
\input{latex/app/result}
